# Supplementary material for: Serverless Data Science -- Are We There Yet? A Case Study of Model Serving
Source: arXiv:2103.02958 source file (2022-03-01)
Supplement: Supplementary file 1 [file appendix.tex]

\section*{Appendix}

Move the clear version of figures here.
